# Supplementary material for: Social Mechanism Design: Making Maximally Acceptable Decisions
Source: arXiv:2211.08501 source file (2023-10-10)
Supplement: Supplementary file 1 [file AAAI2024_appendix.tex]

\setcounter{secnumdepth}{1}

\section{Generic Mechanisms}\label{app:generic}
% Mechanism, Theorem, and proof for consequentialists

\begin{mechanism}[h!]
\caption{\small Max Acceptance with Consequentialists}
\label{alg:Abs_Conseq}
\begin{algorithmic} 
\REQUIRE $(V, \mathcal{R}, \mathcal{Y}, \mathcal{D}_N)$ 

\STATE $\mathcal{Y} \gets \{\bigcup_{i \in N} Y_i\} \bigcap \mathcal{Y}$
\IF{$\mathcal{Y} \neq \emptyset$}
    \FOR{$a \in \mathcal{Y}$}
        \STATE $N^a \gets |\{i \in N: a \in Y_i\}|$
        \STATE $R^a = \emptyset$
    \ENDFOR
\ENDIF
\STATE $a^* \gets \argmax\limits_{a \in \mathcal{Y}} N^a$
\FOR{$R \in \mathcal{R}$}
    \STATE $a \gets R(V)$
    \IF{$a = a^*$ or $\mathcal{Y} = \emptyset$}
        \RETURN $(V, R, a)$
    \ELSIF{$a \in \mathcal{Y}$ and $R^a = \emptyset$}
        \STATE $R^a \gets R$
    \ENDIF
\ENDFOR
\STATE $\mathcal{Y} \gets \{a \in \mathcal{Y} : R^a \neq \emptyset\}$
\STATE $y \gets \argmax\limits_{a \in \mathcal{Y}} N^a$
\RETURN $(V, R^y, y)$
\end{algorithmic}
\end{mechanism}

\begin{proposition}
    Mechanism~\ref{alg:Abs_Conseq} maximizes acceptance when all agents are consequentialists.
\end{proposition}

\begin{proof}
    Mechanism~\ref{alg:Abs_Conseq} takes the set of feasible outcomes and removes any outcomes that do not appear in the set $Y_i$ of any agent. If the resulting set is empty, the mechanism returns any feasible decision, though it will not be accepted by any agent. If the set is non-empty, then the algorithm counts for each remaining feasible outcome how many agents have it in their set $Y_i$. The outcome of each feasible rule on the given profile is then computed, and the outcome among them that appeared in the most sets $Y_i$ is returned. This is essentially approval voting using the sets $Y_i$ with the added constraints on feasibility for both rules and outcomes.
\end{proof}

% Mechanism, Theorem, and proof for absolute proceduralists

\begin{algorithm}[h!]
\caption{\small Acceptance Maximization with Abs. Proceduralists}
\begin{algorithmic} \label{alg:Abs_Proc}
\REQUIRE $(V, \mathcal{R}, \mathcal{Y}, \mathcal{D}_N)$ 
\STATE $\mathcal{R} \gets \{\bigcup_{i \in N} R_i\} \bigcap \mathcal{R}$ \qquad \qquad \qquad \text{ (optional)}
\STATE $\mathcal{R} \gets \{R \in \mathcal{R} : R(V) \in \mathcal{Y}\}$
\STATE $R \gets \argmax\limits_{R' \in \mathcal{R}} |\{i \in N: R' \in R_i\}|$
\RETURN $(V, R, R(V))$

\end{algorithmic}
\end{algorithm}

\begin{proposition}
    Mechanism~\ref{alg:Abs_Proc} maximizes acceptance when all agents are absolute proceduralists.
\end{proposition}

\begin{proof}
    Mechanism~\ref{alg:Abs_Proc} uses brute-force search to find the feasible rule that yields a feasible outcome on the given profile and appears in the most sets $R_i$. 
\end{proof}

Mechanism~\ref{alg:Abs_Proc} includes a small, optional step to only consider feasible rules that appear in at least one set $R_i$, which is useful if $\mathcal{R}$ is very large. This should be contrasted with Mechanism~\ref{alg:ADC_Abs_Disj} in the ADC setting in which one does not need to compute the outcome of many rules, because once $N_r$ and $N_p$ are calculated, the outcome under any supermajority rule can be determined in constant time $O(1)$.

% Mechanism, Theorem, and proof for absolute conjunctivists
\begin{mechanism}[h]
\caption{\small Max Acceptance for Abs. Conjunctivists}
\begin{algorithmic} \label{alg:Abs_Conj}
\REQUIRE $(V, \mathcal{R}, \mathcal{Y}, \mathcal{D}_N)$
\STATE $R_i \gets \{R \in R_i : R(V) \in Y_i\}$
\STATE $R = \argmax\limits_{R' \in \mathcal{R}} |\{i \in N : R' \in R_i\}|$
\RETURN $(V, R, R(V))$
\end{algorithmic}
\end{mechanism}

\begin{proposition}
    Mechanism~\ref{alg:Abs_Conj} maximizes acceptance when all agents are absolute conjunctivists.
\end{proposition}

\begin{proof}
    For each agent, Mechanism~\ref{alg:Abs_Conj} removes all rules from $R_i$ that do not select an outcome in $Y_i$ on the given profile. Thus, a rule $R$ is in $R_i$ for agent $i$ if and only if $i$ would accept the decision $(V, R, R(V))$. The mechanism then finds the rule that is in the set $R_i$ of the largest number of agents.
\end{proof}

\section{Asymmetric Dichotomous Choice Acceptance Rate Lower Bounds}\label{app:ADC_bounds}

\begin{proposition}\label{prop:ADC_empty}
    $\alpha_\mathcal{I} = 0$ for the class of all asymmetric dichotomous choice instances.
\end{proposition}

\begin{proof}
    Proposition \ref{prop:ADC_empty} follows simply because if $|R_i| = |Y_i| = 0$ for all agents $i$, then we have a degenerate case where no agent accepts any decision and $\alpha_I = 0$.
\end{proof}

\begin{proposition}\label{prop:ADC_abs_conj_0}
    For any set of absolute conjunctivist agents, if $v_i \in Y_i$ and $|R_i \cap \mathcal{R}| \geq 1$ for all $i \in N$, then $\alpha_\mathcal{I} = 0$ for the class of asymmetric dichotomous choice instances.
\end{proposition}

\begin{proof}
    Even if we assume that for all absolute consequentialist agents there is at least one feasible rule in $R_i$, and that their set $Y_i$ contains their vote $v_i$, it is still possible that no agent accepts any feasible decision on a given profile because there is no feasible rule $R \in R_i$ such that $R(V) \in Y_i$.
\end{proof}

Proposition \ref{prop:ADC_abs_conj_2} says that if all agents are absolute conjunctivists, then even if every agent accepts at least one feasible decision, there still might be no feasible decision that more than 2 agents accept.

\begin{proposition}\label{prop:ADC_abs_conj_2}
    For any set of absolute conjunctivist agents, if $|Y_i \cap \mathcal{Y}| \geq 1$ and $\exists R \in R_i \cap \mathcal{R} : R(V) \in Y_i \cap \mathcal{Y}$ for all $i \in N$, then $\alpha_\mathcal{I} = \frac{2}{n}$ for the class of asymmetric dichotomous choice problems.
\end{proposition}

\begin{proof}
    Let $\tilde{R}_i = \{R \in R_i \cap \mathcal{R} : R(V) \in Y_i \cap \mathcal{Y}\}$ be the subset of feasible rules in $R_i$ that select a feasible outcome on the given profile $V$ that is within $Y_i$. Thus, the absolute conjunctivist agent $i$ will accept a decision $(V, R, R(V))$ if and only if $R \in \tilde{R}_i$. Are assumption states that $\tilde{R}_i$ is non-empty for all agents. With $|\mathcal{R}| = \floor{\frac{n+1}{2}}$ feasible rules and $n$ agents, our bound of $\alpha_\mathcal{I} \geq \frac{2}{n}$ follows by the pigeonhole principle (with $n$ pigeons and $\floor{\frac{n+1}{2}}$ holes). So there must be at least two agents who accept a decision that uses the same rule.
\end{proof}

\begin{corollary}\label{thm:ADC_cons}
    For any set of consequentialists agents, if $|Y_i \cap \mathcal{Y}| \geq 1$ for all $i \in N$, then $\alpha_\mathcal{I} = \frac{1}{2}$ for the class of asymmetric dichotomous choice problems.
\end{corollary}

\begin{proof}
    The lower bound follows from Theorem \ref{thm:II_all} because consequentialists are implementation-indifferent.
    In asymmetric dichotomous choice, $\mathcal{Y} = \{r,p\}$. With $n$ agents for all of whom $Y_i$ contains at least one feasible outcome, either $r$ or $p$ must appear in $Y_i$ of at least half of the agents, by the pigeonhole principle (with $n$ pigeons and $2$ holes). Since all agents are consequentialists, either a decision of the form $(V_{rp}, \_\_, r)$ or $(V_{rp}, \_\_, p)$ must be accepted by at least half the agents, regardless of the rule used, so $\alpha_\mathcal{I} \geq \frac{1}{2}$.
    In the worst case, $|Y_i| = 1$ for all agents, $n$ is even, and exactly half the agents have $Y_i = \{r\}$ while the other half have $Y_i = \{p\}$, so $\alpha_\mathcal{I} \leq \frac{1}{2}$.
\end{proof}

\begin{proposition}\label{prop:ADC_abs_disj_1}
    For any set of absolute disjunctivist agents, if $|R_i \cap \mathcal{R}| \geq 1$ for all $i \in N$, then $\alpha_\mathcal{I} = \frac{2}{n}$ for the class of asymmetric dichotomous choice problems.
\end{proposition}

\begin{proof}
    With $n$ absolute disjunctivist agents, all of whom have at least one feasible rule in their set $R_i$, and $|\mathcal{R}| = \floor{\frac{n+1}{2}}$ feasible rules, there must be at least 2 agents $i,j \in N$ such that $|R_i \cap R_j| \geq 1$ by the pigeonhole principle (with $n$ pigeons and $\floor{\frac{n+1}{2}}$ holes). Therefore $\alpha_\mathcal{I} \geq \frac{2}{n}$, because we can always find some decision $(V, R, R(V))$ accepted by at least two agents. However, there may be no rule accepted by 3 or more agents, and so $\alpha_\mathcal{I} < \frac{3}{n}$.
\end{proof}

\begin{proposition}\label{prop:ADC_abs_disj_k}
    For any set of absolute disjunctivist agents, if $|R_i \cap \mathcal{R}| \geq k$ for all $i \in N$, then $\alpha_\mathcal{I} = \frac{1}{n} \cdot \ceil{\frac{nk}{\floor{\frac{n+1}{2}}}}$ for the class of asymmetric dichotomous choice problems.
\end{proposition}

\begin{proof}
    With $n$ absolute disjunctivist agents all with at least $k$ feasible rules out of the $\floor{\frac{n+1}{2}}$ possible feasible rules in their sets $R_i$, the bound follows from the pigeonhole principle (with $nk$ pigeons and $|\mathcal{R}| = \floor{\frac{n+1}{2}}$ holes) which sets a tight lower bound on the minimum number of agents that must have the same rule in their sets $R_i$.
\end{proof}

\begin{corollary}\label{prop:ADC_abs_disj_y1}
    For any set of absolute disjunctivist agents, if $|Y_i \cap \mathcal{Y}| \geq 1$ for all $i \in N$, then $\alpha_\mathcal{I} = \frac{1}{2}$ for the class of asymmetric dichotomous choice problems.
\end{corollary}

\begin{proof}
    The proof follows from Corollary \ref{thm:ADC_cons}, because consequentialists are a sub-type of absolute disjunctivists. If the agents' rule sets $R_i$ are non-empty, this could only increase $\alpha_\mathcal{I}$.
\end{proof}

The following five corollaries follow directly from Proposition \ref{prop:II_all}, which applies to all sets of II agents, because $\mathcal{Y} = 2$ in asymmetric dichotomous choice problems.

\begin{corollary}\label{prop:ADC_II_conj_1}
    For any set of II-conjunctivist agents, if $|Y_i \cap \mathcal{Y}| \geq 1$ $\exists R \in R_i : R(V) \in \mathcal{Y}$ for all $i \in N$, then $\alpha_\mathcal{I} = \frac{1}{2}$ for the class of asymmetric dichotomous choice problems.
\end{corollary}

\begin{corollary}\label{prop:ADC_II_disj_r1}
    For any set of II-disjunctivist agents, if $\exists R \in R_i : R(V) \in \mathcal{Y}$ for all $i \in N$, then $\alpha_\mathcal{I} = \frac{1}{2}$ for the class of asymmetric dichotomous choice problems.
\end{corollary}

\begin{corollary}\label{prop:ADC_II_disj_y1}
    For any set of II-disjunctivist agents, if $|Y_i \cap \mathcal{Y}| \geq 1$ for all $i \in N$, then $\alpha_\mathcal{I} = \frac{1}{2}$ for the class of asymmetric dichotomous choice problems.
\end{corollary}

\begin{corollary}\label{prop:ADC_II_disj_y1r1}
    For any set of II-disjunctivist agents, if $|Y_i \cap \mathcal{Y}| \geq 1$ and $\exists R \in R_i : R(V) \in \mathcal{Y} \backslash Y_i$ for all $i \in N$, then $\alpha_\mathcal{I} = \frac{1}{2}$ for the class of asymmetric dichotomous choice problems.
\end{corollary}

% \begin{proposition}\label{prop:ADC_abs_disj_vyr1}
%     For any set of absolute disjunctivist agents, if $v_i \in Y_i$ and $|R_i \cap \mathcal{R}| \geq 1$ for all $i \in N$, then $\alpha_\mathcal{I} = \frac{1}{2}$ for the class of asymmetric dichotomous choice problems.
% \end{proposition}

\paragraph{Consequentialists}
Suppose all agents are consequentialists and their satisfying sets are \emph{consistent} with their votes $v_i \in \{r,p\}$ such that $v_i \in Y_i$ and $\mathcal{D}_i = \{(V, R, y) \in \mathcal{D} : y \in Y_i\}$ for all $i \in N$.
Universal acceptance with consequentialists is only possible if there is an outcome everyone accepts: $\bigcap\limits_{i \in N} Y_i \neq \emptyset$. The worst-case acceptance rate is determined by the minimum size of the majority, which is half the agents. 

\begin{proposition}\label{prop_adc_abs_conseq_consistent}
 For asymmetric dichotomous choice with all consequentialist agents such that $v_i \in Y_i$, the worst-case acceptance rate is $\alpha_\mathcal{I} = \frac{1}{2}$, which is achieved by the simple mechanism $M$ that applies majority rule $R^{\frac{1}{2}}$ to the profile $V$ in every instance.
\end{proposition}

\begin{proof}
The proof of the lower bound of $\frac{1}{2}$ on $\alpha_\mathcal{I}$ in Proposition \ref{prop_adc_abs_conseq_consistent} follows from the pigeonhole principle. One of the two potential outcomes, $r$ or $p$, must be accepted by at least half of the agents because we forbid abstention and empty satisfying sets. This follows from the requirement that $v_i \in Y_i$. With $n$ pigeons and $2$ holes there must be at least $\ceil{\frac{n}{2}}$ pigeons in one of the holes. Therefore, for any instance, we can always achieve an acceptance rate of at least $\frac{1}{2}$ by making the decision according to majority rule: $(V, R^\frac{1}{2}, R^\frac{1}{2}(V))$.

In the worst case, $Y_i = \{v_i\}$ for every agent $i \in N$, the number of agents $n$ is even, and exactly half of the agents vote for each alternative. Any feasible decision satisfies exactly half of the agents, so we know $\alpha_\mathcal{I} \leq \frac{1}{2}$ because no mechanism can achieve a higher acceptance rate on this instance. This gives us our upper bound of $\frac{1}{2}$.
\end{proof}

Notice that the mechanism $M$ in Proposition \ref{prop_adc_abs_conseq_consistent} does not maximize acceptance for every instance. A decision with the alternative that receives fewer votes as its outcome might still be acceptable to a greater fraction of the agents. However, the proof above shows that the mechanism $M$ that maximizes acceptance must also have $\alpha_\mathcal{I} = \frac{1}{2}$.
The same value of $\alpha_\mathcal{I} = \frac{1}{2}$ is obtained for the smaller class of instances with the stronger requirement that $Y_i = \{v_i\}$ for all agents. The proof is essentially the same as the one above. 
If agents can be inconsistent, where $v_i \not \in Y_i$, then $\alpha_\mathcal{I} = 0$ because of the degenerate instances where $v_i = r$ and $Y_i = \{p\}$ for all $i \in N$.

\paragraph{Absolute Proceduralists}
Suppose every agent has a vote $v_i \in \{r,p\}$ and a set of one or more supermajority rules $R_i \subseteq \mathcal{R}$ such that $(V, R, y) \in \mathcal{D}_i$ if and only if $R \in R_i$.
The optimal mechanism counts for each supermajority rule $R$ the number of sets $R_i$ that contain $R$ and then picks among these rules the one with the highest count. The outcome is uniquely determined by the choice of rule and the profile.
For there to be universal acceptance, it would have to be that $\bigcap\limits_{i \in N} R_i \neq \emptyset$. 

\paragraph{II-conjunctivists}
An acceptance maximizing mechanism for II-conjunctivists can be created by changing the `or' to `and' in lines 3 and 4 of Mechanism~\ref{alg:II_binary} defining $N_r$ and $N_p$.

% Proof for each row of table

% Each of the four types described so far are examples of absolutism.

% \begin{definition}[Absolutism]
% Agent $i \in N$ is absolutist if for all decisions $(V, R, y)$, $(V', R, y) \in \mathbb{D}$, we have $(V, R, y) \in \mathcal{D}_i \Rightarrow (V', R, y) \in \mathcal{D}_i$
% \end{definition}
